# Supplementary material for: Federated Self-supervised Learning for Heterogeneous Clients
Source: arXiv:2205.12493 source file (2022-05-31)
Supplement: Supplementary file 1 [file appendix.tex]

\subsection{Proof of Lemma~\ref{local_epochs}}
\label{sec:proof:local_epochs}
Let $\mathcal{L}_{E}$ denote the loss function after $E$ local epochs. \\ \\
$ \mathcal{L}_{1} \leq \mathcal{L}_{0} - \eta  [\nabla \mathcal{L}_{0}^T g_0] + \dfrac{L_1 \eta^2}{2} [||g_0||^2] $ \\ \\
$ \E [\mathcal{L}_{1}] \leq \E[\mathcal{L}_{0}] - \eta \E [\nabla \mathcal{L}_{0}^T g_0] + \dfrac{L_1 \eta^2}{2} \E[||g_0||^2] $ \\ \\
$ \hspace*{0.25in} = \E[\mathcal{L}_{0}] - \eta ||\nabla \mathcal{L}_{0} ||^2 + \dfrac{L_1 \eta^2}{2} \E[||g_0||^2] $ \\ \\
$ \hspace*{0.25in} = \E[\mathcal{L}_{0}] - \eta ||\nabla \mathcal{L}_{0} ||^2 + \dfrac{L_1 \eta^2}{2} (Var(g_0) + \E[||g_0||]^2) $ \\ \\
$ \hspace*{0.25in} \leq \E[\mathcal{L}_{0}] - (\eta - \dfrac{L_1 \eta^2}{2}) ||\nabla \mathcal{L}_{0} ||^2 + \dfrac{L_1 \eta^2}{2} \sigma^2 $ \\ \\
Summing for $E$ number of local epochs, \\ \\
$\sum_{i=1}^{E} \E[\mathcal{L}_{i}] \leq \sum_{i=0}^{E-1} \E[\mathcal{L}_{i}] - (\eta - \dfrac{L_1 \eta^2}{2})\sum_{i=0}^{E-1}||\nabla \mathcal{L}_{i} ||^2 + \dfrac{L_1 E \eta^2}{2} \sigma^2 $ \\ \\
$ \E[\mathcal{L}_{E}] \leq  \mathcal{L}_{0} - (\eta - \dfrac{L_1 \eta^2}{2})\sum_{i=0}^{E-1}||\nabla \mathcal{L}_{i} ||^2 + \dfrac{L_1 E \eta^2}{2} \sigma^2 $ \\ \\
Thus if $\eta < \dfrac{2(\sum_{i=0}^{E-1}||\nabla \mathcal{L}_{i} ||^2)}{L_1 (\sum_{i=0}^{E-1} ||\nabla \mathcal{L}_{i} ||^2 + E \sigma^2)}$, \\ \\
$\mathcal{L}_{E} \leq  \mathcal{L}_{0}$ and the local loss reduces after $E$ local epochs.
\subsection{Proof of Lemma~\ref{rep_update}}
\label{sec:proof:rep_update}

For any arbitrary client \\ 

$\loss_{E'} = \loss_E + \loss_{E'} - \loss_E$ \\ 

\hspace*{0.25in} $ = \loss_E + \mu \bl \loss^{\text{proximal}}_{E'} - \loss^{\text{proximal}}_E \br$ \\ 

If $\loss^{\text{proximal}} = || \Phi ( \X ; \W^{(t)} ) - \Bar{\Phi}(\X;(t-1))|| $, \\ 

$\loss_{E'} = \loss_E + \mu \bl || \Phi ( \X ; \W^{(t)} ) - \Bar{\Phi}(\X;(t))|| \br - \mu \bl || \Phi ( \X ; \W^{(t)} ) - \Bar{\Phi}(\X;(t-1))|| \br$ \\ 

\hspace*{0.25in} $ \leq \loss_E +  \mu \bl || \Bar{\Phi}(\X;(t))|| - \Bar{\Phi}(\X;(t-1))|| \br$ \\ 

\hspace*{0.25in} $ = \loss_E +  \mu \bl || \sum_{k=1}^{N} w_k \Phi_k ( \X ; \W_k^{(t)} ) - \sum_{k=1}^{N} w_k \Phi_k ( \X ; \W_k^{(t-1)} )|| \br$ \\ 

\hspace*{0.25in} $ \leq \loss_E +  \mu \bl \sum_{k=1}^{N} w_k || \Phi_k ( \X ; \W_k^{(t)} ) -  \Phi_k ( \X ; \W_k^{(t-1)} )|| \br$ \\ 

\hspace*{0.25in} $ \leq \loss_E +  \mu \bl \sum_{k=1}^{N} w_k || \Phi_k ( \X ; \W_k^{(t)} ) - \sum_{k=1}^{N} w_k \Phi_k ( \X ; \W_k^{(t-1)} )|| \br$ \\ 

\hspace*{0.25in} $ \leq \loss_E +  \mu L_2 \bl \sum_{k=1}^{N} w_k || \W_k^{(t)} - \W_k^{(t-1)} ||\br$ \\ 

\hspace*{0.25in} $ = \loss_E  + \mu L_2 \bl \sum_{k=1}^{N} w_k || \sum_{e=1}^{E} \eta g_{k}^{(te)}|| \br$ \\ 

\hspace*{0.25in} $ = \loss_E  + \mu L_2 \bl \sum_{k=1}^{N} w_k || \sum_{e=1}^{E} \eta g_{k}^{(te)}|| \br$ \\ 

\hspace*{0.25in} $ \leq \loss_E  + \mu L_2 \bl \sum_{k=1}^{N} w_k \sum_{e=1}^{E} \eta || g_{k}^{(te)}|| \br$ \\ 

\hspace*{0.25in} $ = \loss_E + \mu L_2 \eta \bl \sum_{k=1}^{N} w_k \sum_{e=1}^{E}  || g_{k}^{(te)}|| \br$ \\ 

Taking expectation on both sides, \\
$\E [\loss_{E'}] \leq \E[\loss_E] + \mu L_2 \eta \bl \sum_{k=1}^{N} w_k \sum_{e=1}^{E} \E[|| g_{k}^{(te)}||] \br$ \\ 

$\E [\loss_{E'}] \leq \loss_E + \mu L_2 \eta E P$ \\ 

On the other hand, if $\loss^{\text{proximal}} = \cka(K_i(t), \Bar{K}(t-1)) $, we have  \\ 

$\loss_{E'} = \loss_E + \mu \bl \cka(K_i(t), \Bar{K}(t)) - \cka(K_i(t), \Bar{K}(t-1)) \br$ \\ 

\hspace*{0.25in} $ = \loss_E + \mu \bl \text{trace}(K_i(t) \Bar{K}(t)) - \text{trace}(K_i(t) \Bar{K}(t-1)) \br$ \\ 

\hspace*{0.25in} $ = \loss_E + \mu \bl \text{trace}(K_i(t) (\Bar{K}(t) - \Bar{K}(t-1))) \br$ \\ 

\hspace*{0.25in} $ = \loss_E + \mu \bl \text{trace} (K_i(t) (\sum_{k=1}^{N} w_k K_k(t) - \sum_{k=1}^{N} w_k K_k(t-1) ) \br$ \\ 

\hspace*{0.25in} $ = \loss_E + \mu \bl \sum_{i=1}^{L} \sum_{j=1}^{L} (K_i(t)_{i,j} (\sum_{k=1}^{N} w_k K_k(t)_{i,j} - \sum_{k=1}^{N} w_k K_k(t-1)_{i,j} ) \br$ \\ 

\hspace*{0.25in} $ = \loss_E + \mu \bl \sum_{k=1}^{N} w_k( \sum_{i=1}^{L} \sum_{j=1}^{L} K_i(t)_{i,j} ( K_k(t)_{i,j} -  K_k(t-1)_{i,j} )) \br$ \\ 

\hspace*{0.25in} $ = \loss_E + \mu \bl \sum_{k=1}^{N} w_k( \sum_{i=1}^{L} \sum_{j=1}^{L} K_i(t)_{i,j} ( \Phi_k(x_i; \W_k^t) . \Phi_k(x_j; \W_k^t) - \Phi_k(x_i; \W_k^{t-1}) . \Phi_k(x_j; \W_k^{t-1}) )) \br$ \\ 

\hspace*{0.25in} $ = \loss_E + \mu \sum_{k=1}^{N} w_k \sum_{i=1}^{L} \sum_{j=1}^{L} K_i(t)_{i,j} \bl \Phi_k(x_i; \W_k^{t}) (\Phi_k(x_j; \W_k^{t}) - \Phi_k(x_j; \W_k^{t - 1})) + \Phi_k(x_j; \W_k^{t - 1})(\Phi_k(x_i; \W_k^{t})  -  \Phi_k(x_i; \W_k^{t-1})) \br$ \\

Taking norm on both the sides, \\ 

$||\loss_{E'}|| = ||\loss_E + \mu \sum_{k=1}^{N} w_k \sum_{i=1}^{L} \sum_{j=1}^{L} K_i(t)_{i,j} \bl \Phi_k(x_i; \W_k^{t}) (\Phi_k(x_j; \W_k^{t}) - \Phi_k(x_j; \W_k^{t - 1})) + \Phi_k(x_j; \W_k^{t - 1})(\Phi_k(x_i; \W_k^{t})  -  \Phi_k(x_i; \W_k^{t-1})) \br|| $ \\

$\loss_{E'} \leq ||\loss_E|| + \mu ||\sum_{k=1}^{N} w_k \sum_{i=1}^{L} \sum_{j=1}^{L} K_i(t)_{i,j} \bl \Phi_k(x_i; \W_k^{t}) (\Phi_k(x_j; \W_k^{t}) - \Phi_k(x_j; \W_k^{t - 1})) + \Phi_k(x_j; \W_k^{t - 1})(\Phi_k(x_i; \W_k^{t})  -  \Phi_k(x_i; \W_k^{t-1})) \br|| $ \\

\hspace*{0.25in} $ \leq \loss_E + \mu \sum_{k=1}^{N} w_k \sum_{i=1}^{L} \sum_{j=1}^{L} ||K_i(t)_{i,j}||  \bl ||\Phi_k(x_i; \W_k^{t}) (\Phi_k(x_j; \W_k^{t}) - \Phi_k(x_j; \W_k^{t - 1})) + \Phi_k(x_j; \W_k^{t - 1})(\Phi_k(x_i; \W_k^{t})  -  \Phi_k(x_i; \W_k^{t-1}))|| \br $ \\

\hspace*{0.25in} $ \leq \loss_E + \mu \sum_{k=1}^{N} w_k \sum_{i=1}^{L} \sum_{j=1}^{L} ||K_i(t)_{i,j}|| \bl ||\Phi_k(x_i; \W_k^{t}) (\Phi_k(x_j; \W_k^{t}) - \Phi_k(x_j; \W_k^{t - 1}))|| + ||\Phi_k(x_j; \W_k^{t - 1})(\Phi_k(x_i; \W_k^{t})  -  \Phi_k(x_i; \W_k^{t-1}))|| \br $ \\

\hspace*{0.25in} $ \leq \loss_E + \mu \sum_{k=1}^{N} w_k \sum_{i=1}^{L} \sum_{j=1}^{L} ||K_i(t)_{i,j}|| \bl ||\Phi_k(x_i; \W_k^{t})||. ||(\Phi_k(x_j; \W_k^{t}) - \Phi_k(x_j; \W_k^{t - 1}))|| + ||\Phi_k(x_j; \W_k^{t - 1})||.||(\Phi_k(x_i; \W_k^{t})  -  \Phi_k(x_i; \W_k^{t-1}))|| \br $ \\

\hspace*{0.25in} $ \leq \loss_E + \mu \sum_{k=1}^{N} w_k \sum_{i=1}^{L} \sum_{j=1}^{L} ||K_i(t)_{i,j}|| \bl ||\Phi_k(x_i; \W_k^{t})||. ||\text{L}_2 \eta g_{t,k}|| + ||\Phi_k(x_j; \W_k^{t - 1})||.||\text{L}_2 \eta g_{t,k}|| \br $ \\

$\E[\loss_{E'}] \leq \E[\loss_E] + \mu \sum_{k=1}^{N} w_k \sum_{i=1}^{L} \sum_{j=1}^{L} \E[ ||K_i(t)_{i,j}|| \bl ||\Phi_k(x_i; \W_k^{t})||. ||\text{L}_2 \eta g_{t,k}||] + \E[||\Phi_k(x_j; \W_k^{t - 1})||.||\text{L}_2 \eta g_{t,k}||] $ \\

\hspace*{0.25in} $ \leq \E[\loss_E] + \mu \sum_{k=1}^{N} w_k \sum_{i=1}^{L} \sum_{j=1}^{L} ||K_i(t)_{i,j}|| \bl R \text{L}_2 \eta P  + R \text{L}_2 \eta P \br $ \\

\hspace*{0.25in} $ = \E[\loss_E] + 2 \mu \eta \text{L}_2 P R \sum_{i=1}^{L} \sum_{j=1}^{L} ||K_i(t)_{i,j}||   $ \\

\hspace*{0.25in} $ \leq \E[\loss_E] + 2 \mu \eta \text{L}_2 P R \sum_{i=1}^{L} \sum_{j=1}^{L} R^2   $ \\

\hspace*{0.25in} $ \leq \E[\loss_E] + 2 \mu \eta \text{L}_2 P R^3 L^2 $ \\

$\E[\loss_{E'}] \leq \E[\loss_E] + 2 \mu \eta \text{L}_2 P R^3 L^2 $.

\section{Additional Experiments}
\label{sec:additional_experiments}
\begin{table}[!htb]
  \caption{Test Accuracy of various federated self-supervised methods with change in scale on CIFAR-10 dataset}
  \label{scalable_c10}
  \centering
  \begin{tabular}{lcr}
    \toprule
    \cmidrule(r){1-2}
    Dataset  &  5clients(5) &  20clients(5)  \\
    \midrule
    FedU        & 79.6 $\pm$ 0.5   &  82.52 $\pm$ 1.2  \\
    FedEMA      & 81.2 $\pm$ 1.6   &  83.17 $\pm$ 0.7   \\
    Hetero-SSFL & 90.29 $\pm$ 0.3  &  89.2  $\pm$ 0.65  \\
    \bottomrule
  \end{tabular}
\end{table}
